# Supplementary material for: Online Coresets for Clustering with Bregman Divergences
Source: arXiv:2012.06522 source file (2020-12-11)
Supplement: Supplementary file 1 [file appendix.tex]

\section{Appendix}{\label{sec:appendix}}
Before we discuss the proofs of the supporting lemmas and arguments, we state definition and theorems that are useful in the discussion.
\paragraph{Well-Conditioned Basis:\label{defi:wellConditionedBais}}\cite{dasgupta2009sampling}Let $\*A \in \~R^{n \times d}$ a rank $d$ matrix. For $p \geq 1$, it has a dual $q = p/(p-1)$. A matrix $\*U$ is said to be $(\alpha,\beta,p)$ \emph{well-conditioned basis} of $\*A$, if $\*U$ spans the column space of $\*A$, $\sum_{i=1}^{d}\|\*u_{j}\|_{p}\leq \alpha$, $\forall \*x \in \~R^{d}, \frac{\|\*x\|_{q}}{\|\*U\*x\|_{p}}\leq \beta$ and $(\alpha, \beta)$ are $d^{O(1)}$ and also independent of $n$.
\begin{theorem}{\label{thm:bernstein}}
\textbf{Bernstein \cite{dubhashi2009concentration}} Let the scalar random variables $x_{1}, x_{2}, _{\cdots}, x_{n}$ be independent that satisfy $\forall i \in [n]$,  
$\vert x_{i}-\~E[x_{i}]\vert \leq b$. 
Let $X = \sum_{i} x_{i}$ and let $\sigma^{2} = \sum_{i} \sigma_{i}^{2}$ be the variance of $X$. 
Then for any $t>0$,
\begin{center}
 $\mbox{Pr}\big(X > \~E[X] + t\big) \leq \exp\bigg(\frac{-t^{2}}{2\sigma^{2}+bt/3} \bigg)$
\end{center}
\end{theorem}
\begin{theorem}{\label{thm:matrixBernstein}}
 \textbf{Matrix Bernstein\cite{tropp2015introduction}} Let $\*X_{1},\ldots,\*X_{n}$ are independent $d \times d$ random matrices such that $\forall i \in [n], \|\*X_{i}\|] \leq b$ and $\mbox{var}(\|\*X\|) \leq \sigma^{2}$ where $\*X = \sum_{i=1}^{n}\*X_{i}$, then for some $t>0$,
 $$\mbox{Pr}(\|\*X\| - \~E[\|\*X\|] \geq t) \leq d\exp(\frac{-t^{2}/2}{\sigma^{2}+bt/3})$$
\end{theorem}
\begin{lemma}{\label{lemma:modified-SM}}
 Given a rank-k positive semi-definite matrix $\*M \in \~R^{d \times d}$ and a vector $\*x$ such that it completely lies in the column space of $\*M$. Then we have,
 $$(\*M + \*x\*x^{T})^{\dagger} = \*M^{\dagger} - \frac{\*M^{\dagger}\*x\*x^{T}\*M^{\dagger}}{1+\*x^{T}\*M^{\dagger}\*x} $$
\end{lemma}
\begin{proof}
 The proof is in the similar spirit to lemma \ref{lemma:onlineSummationBound}. Consider $[\*V\Sigma,\*V] = \mbox{SVD}(\*M)$ and since $\*x$ lies completely in the column space of $\*M$, hence $\exists \*y \in \~R^{k}$ such that $\*V\*y = \*x$. Note that $\*V \in \~R^{d \times k}$.
 \begin{eqnarray*}
  (\*M + \*x\*x^{T})^{\dagger} &=& (\*V\Sigma\*V^{T}+\*V\*y\*y^{T}\*V^{T})^{\dagger} \\
  &=& \*V(\Sigma+\*y\*y^{T})^{-1}\*V^{T} \\
  &=& \*V\bigg(\Sigma^{-1} - \frac{\Sigma^{-1}\*y\*y^{T}\Sigma^{-1}}{1+y^{T}\Sigma^{-1}\*y}\bigg)\*V \\
  &=& \*V\bigg(\Sigma^{-1}-\frac{\Sigma^{-1}\*V^{T}\*V\*y\*y^{T}\*V^{T}\*V\Sigma^{-1}}{1+y^{T}\*V^{T}\*V\Sigma^{-1}\*V^{T}\*V\*y}\bigg)\*V\\
  &=& \*M^{\dagger} - \frac{\*M^{\dagger}\*x\*x^{T}\*M^{-1}}{1+\*x\*M^{\dagger}\*x}
 \end{eqnarray*}
 The third equality is by Sherman Morrison Formula.
\end{proof}
\noindent\textbf{$\epsilon$-net argument:}{\label{argument:epsNet}} Note that $\norm{\Pi \*A\*x}_{p}^{p} = \sum_{i=1}^{m} |\tilde{\*a}_{i}^{T}\*x|^{p}$, where $\Pi$ is a sampling matrix which samples $m$ rows from $\*A$ with proper scaling. Now we argue this $\forall \*x \in \*C$, i.e. $\norm{\Pi \*A\*x}_{p}^{p} = (1\pm\epsilon)\norm{\*A\*x}_{p}^{p}$ which is same as $\norm{\Pi \*U\*y}_{p}^{p} = (1\pm\epsilon)\norm{\*U\*y}_{p}^{p}$ where $\*U\*y=\*A\*x$. Now with an $\epsilon-$net, we argue $\forall \*x \in \*C$, $\*C \subseteq \~R^{d}$. 

Let $\mcal B = \{ \*z \in \~R^{n} \vert \*z = \*U\*y \mbox{ for some } y \in \~R^{k} \mbox{ and } \norm{\*z}_{p} = 1 \}$. From this set we intend to find a finite subset $\mcal N$ which is an $\epsilon$-net to the set. Now here we argue that if we can ensure $\norm{\Pi \*w}_{p}^{p} = (1\pm\epsilon)\norm{\*w}_{p}^{p}, \forall \*w \in \mcal N$ then we can claim that $\norm{\Pi \*z}_{p}^{p} = (1\pm\epsilon)\norm{\*z}_{p}^{p}, \forall \*z \in \mcal B$ which further imply that $\norm{\Pi \*A\*x}_{p}^{p} = (1\pm\epsilon)\norm{\*A\*x}_{p}^{p}, \forall \*x \in \*C$.

Let $\*v \in \mcal B$ whose closest $\epsilon$-net point is $\*w_{1} \in \mcal N$ such that $\norm{\*v - \*w_{1}}_{p} \leq \epsilon$. Now note that,
\begin{eqnarray*}
 \norm{\Pi \*v}_{p}^{p} &=& \norm{\Pi \*w_{1} + \Pi(\*v-\*w_{1})}_{p}^{p} \nonumber \\
 &\leq& (\norm{\Pi \*w_{1}}_{p} + \norm{\Pi(\*v-\*w_{1})}_{p})^{p} \nonumber \\
 &\leq& (1+\epsilon + \norm{\Pi(\*v-\*w_{1})}_{p})^{p} \nonumber \\
 &=& (1+\epsilon + \norm{\Pi(\*w_{2}/\alpha + \*v-\*w_{1}-\*w_{2}/\alpha)}_{p})^{p} \nonumber \\
 &\leq& (1+\epsilon + \epsilon(1+\epsilon) + \norm{\Pi(\*v-\*w_{1}-\*w_{2}/\alpha)}_{p})^{p}
\end{eqnarray*}
Repeated application of this argument yields
\begin{center}
 $\norm{\Pi \*v}_{p}^{p} \leq \bigg(\sum_{i\geq0} (1+\epsilon)\epsilon^{i}\bigg)^{p} \leq \bigg(\frac{1+\epsilon}{1-\epsilon}\bigg)^{p} \leq 1 + \mcal O(\epsilon)$ 
\end{center}
By similar argument one can show that $\norm{\Pi \*v}_{p}^{p} \geq 1 - \mcal O(\epsilon)$. Finally by rescaling $\epsilon$ by some constant factor we achieve $\norm{\Pi \*z}_{p}^{p} \in 1\pm\epsilon, \forall \*z \in \mcal B$.
\begin{lemma}{\label{lemma:netSize}}
 There is an $\epsilon$-net $\mcal N$, with $\vert\mcal N\vert \leq (2/\epsilon)^{k}$.
\end{lemma}
\begin{proof}
Let $\mcal N$ be the maximal subset of $\*y \in \~R^{n}$ in the column space of $\*A$ such that $\norm{\*y}_{p} = 1$ and $\forall \*y \neq \*y' \in \mcal N, \norm{\*y-\*y'}_{p} > \epsilon$. Now as $\mcal N$ is a maximal set, hence $\forall \*y \in \mcal B, \exists \*w \in \mcal N$ for which $\norm{\*w-\*y}_{p} \leq \epsilon$. Further $\forall \*y \neq \*y' \in \mcal N$ two balls centered at $\*y$ and $\*y'$ with radius $\epsilon/2$ are disjoint otherwise by triangle inequality, $\norm{\*y-\*y'}_{p} \leq \epsilon$, is a contradiction. So it follows that in a unit sphere in $\~R^{k}$ there could be at most $(2/\epsilon)^{k}$ such balls, i.e. the number of points in $\mcal N$. 
\end{proof}
% 
% \subsubsection{Proof of Lemma \ref{lemma:offlineSummationBound}}
% \begin{proof}{\label{proof:summationBound}}
%  We know that $\sum_{i=1}^{n} \norm{u_{i}}^{2} = d$. Let the upper bound to an $S_{i}$ is $l_{i} = \min\{1,n^{p/2-1}\norm{u_{i}}^{p}\}$.  There are two cases that decide the value of $l_{i}$. When $\norm{u_{i}}^{p} \geq n^{1-p/2}$ then $l_{i} = 1$, this implies that $\norm{u_{i}}^{2} \geq n^{2/p-1}$. But we know $\sum_{i=1}^{n}\norm{u_{i}}^{2} = d$ so there are at-most $n^{1-2/p}d$ such $l_{i}$'s. Now for the case where $\norm{u_{i}}^{p} < n^{1-p/2}$, we get $\norm{u_{i}}^{p-2} < (1/n)^{(p/2-1)(1-2/p)}$. Then $\sum_{i=1}^{n} n^{p/2-1}\norm{u_{i}}^{p} = \sum_{i=1}^{n} n^{p/2-1}\norm{u_{i}}^{p-2} \norm{u_{i}}^{2} <\sum_{i=1}^{n}n^{1-2/p}\norm{u_{i}}^{2} = n^{1-2/p}d$.
% \end{proof}
% Note that (eqn \ref{eqn1}) for even $p$ value is same as subspace embedding. \cite{dasgupta2009sampling} shows that there is a sampling algorithm for any $\ell_{p}$ regression. To prove it authors first show that with $O(d^{p+1})$ one can preserve the $p$ norm subspace embedding. Now we discuss the lemmas of online setting.
\subsection{\online}
 Here we provide the proofs of the lemmas used to prove theorem~\ref{thm:Online}.
\subsubsection{Proof of lemma \ref{lemma:onlineSensitivityBound}}
\begin{proof}{\label{proof:onlineSensitivityBound}}
We define the online sensitivity scores $\tilde{s}_{i}$ for each point $i$ as follows,
\begin{center}
 $\tilde{s}_{i} = \sup_{\*x}\frac{\vert \*a_{i}^{T}\*x\vert^{p}}{\sum_{j=1}^{i}\vert \*a_{j}^{T}\*x\vert^{p}} = \sup_{\*y}\frac{\vert \*u_{i}^{T}\*y\vert^{p}} {\sum_{j=1}^{i}\vert \*u_{j}^{T}\*y\vert^{p}}$
\end{center}
Here $\*y = \Sigma \*V^{T}\*x$ where $[\*U,\Sigma,\*V] = \mbox{svd}(\*A)$ and $\*u_{i}^{T}$ is the $i^{th}$ row of $\*U$. Now at this $i^{th}$ step we define $[\*U_{i},\Sigma_{i},\*V_{i}] = \mbox{svd}(\*A_{i})$. So we rewrite the above optimization function as follows with $\*y = \Sigma_{i} \*V_{i}^{T}\*x$ and $\tilde{\*u}_{i}^{T}$ is the $i^{th}$ row of $\*U_{i}$,
\begin{center}
 $\tilde{s}_{i} = \sup_{\*x}\frac{\vert \*a_{i}^{T}\*x\vert^{p}}{\sum_{j=1}^{i}\vert \*a_{j}^{T}\*x\vert^{p}}=\sup_{\*y}\frac{\vert \tilde{\*u}_{i}^{T}\*y\vert^{p}}{\norm{\*U_{i}\*y}_{p}^{p}}=\sup_{\*y}\frac{\vert \tilde{\*u}_{i}^{T}\*y\vert^{p}}{\vert \tilde{\*u}_{i}^{T}\*y\vert^{p}+\sum_{j=1}^{i-1}\vert \tilde{\*u}_{j}^{T}\*y\vert^{p}}$
\end{center}
Let there be an $\*x^{*}$ which maximizes $\tilde{s}_{i}$. Corresponding to it we have  $\*y^{*} = \Sigma_{i} \*V_{i}^{T}\*x^{*}$. For a fixed $\*x$, let $f(\*x) = \frac{\vert \*a_{i}^{T}\*x\vert^{p}}{\sum_{j=1}^{i}\vert \*a_{j}^{T}\*x\vert^{p}}$ and $g(\*y) = \frac{\vert \tilde{\*u}_{i}^{T}\*y\vert^{p}}{\norm{\*U_{i}\*y}_{p}^{p}}$. By assumption we have $f(\*x^{*}) \geq f(\*x), \forall \*x$. We prove by contradiction that its corresponding $g(\*y^{*}) \geq g(\*y), \forall \*y$, where $\*y = \Sigma_{i} \*V_{i}^{T}\*x$. Let $\exists \*y'$ such that $g(\*y') \geq g(\*y^{*})$. Then we get $\*x' = \*V_{i}\Sigma_{i}^{-1}\*y'$ for which $f(\*x') \geq f(\*x^{*})$. This contradicts our assumption, unless $\*x' = \*x^{*}$. To maximize the score $\*x$ are chosen from the row space of $\*A_{i}$. Now without loss of generality we assume that $\norm{\*y} = 1$ and we know that if $\*x$ is in the row space of $\*A_{i}$ then $\*y$ is in the row space of $\*U_{i}$. Hence we get $\norm{\*U_{i}\*y} = \norm{\*y} = 1$.

We break denominator into sum of numerator and the rest, i.e. $\norm{\*U_{i}\*y}_{p}^{p} = \vert \tilde{\*u}_{i}^{T}\*y\vert^{p}+\sum_{j=1}^{i-1}\vert \tilde{\*u}_{j}^{T}\*y\vert^{p}$. % So we have $(\~E[\*a_{i}^{T}b])^{2} \leq \~E[(\*a_{i}^{T}b)^{2}] = \parallel b \parallel^{2}$, i.e. $\~E[\*a_{i}^{T}b] \leq \parallel b \parallel$. Now if $b = \*a_{i}$, then $\~E[\*a_{i}^{T}b] \leq \parallel b \parallel = \sqrt{d}$ and $\*a_{i}^{T}b = d$. The sensitivity score of row $i$ is $(sf(i))$ which is defined as follows,
Consider the denominator term which is $\sum_{j=1}^{i-1}|\tilde{\*u}_{j}^{T}\*y|^{p} \geq \bigg(\sum_{j=1}^{i-1} |\tilde{\*u}_{j}^{T}\*y|^{2}\bigg)\cdot f(n)$. From this we estimate $f(n)$ as follows,
\begin{eqnarray}
\sum_{j=1}^{i-1}|\tilde{\*u}_{j}^{T}\*y|^{2} &=& \bigg(\sum_{j=1}^{i-1}|\tilde{\*u}_{j}^{T}\*y|^{2}\cdot 1\bigg) \nonumber \\
&\leq& \bigg(\sum_{j=1}^{i-1}|\tilde{\*u}_{j}^{T}\*y|^{2\cdot p/2}\bigg)^{2/p}\bigg(\sum_{j=1}^{i-1}1^{p/(p-2)}\bigg)^{1-2/p}\label{eqn:holder1}\\
&\leq& \bigg(\sum_{j=1}^{i-1}|\tilde{\*u}_{j}^{T}\*y|^{p}\bigg)^{2/p}\cdot(i)^{1-2/p} \label{eqn:last1}
\end{eqnarray}
Here equation \eqref{eqn:holder1} is by holder's inequality, where $2/p + 1 - 2/p = 1$. So we rewrite the above term as $\big(\sum_{j=1}^{i-1}|\tilde{\*u}_{j}^{T}\*y|^{p}\big)^{2/p} \big(i\big)^{1-2/p} \geq \sum_{j=1}^{i-1} |\tilde{\*u}_{j}^{T}\*y|^{2} = 1 - |\tilde{\*u}_{i}^{T}\*y|^{2}$. Now substituting this in equation \eqref{eqn:last1} we get,
\begin{eqnarray*}
\bigg(\sum_{j=1}^{i-1}|\tilde{\*u}_{j}^{T}\*y|^{p}\bigg)^{2/p} &\geq& \bigg(\frac{1}{i}\bigg)^{1-2/p} (1 - |\tilde{\*u}_{i}^{T}\*y|^{2})\\
\bigg(\sum_{j=1}^{i-1}|\tilde{\*u}_{j}^{T}\*y|^{p}\bigg) &\geq& \bigg(\frac{1}{i}\bigg)^{p/2-1}(1 - |\tilde{\*u}_{i}^{T}\*y|^{2})^{p/2}
\end{eqnarray*}
So we get $\tilde{s}_{i} \leq \sup_{\*y}\frac{\vert \tilde{\*u}_{i}^{T}\*y\vert^{p}}{\vert \tilde{\*u}_{i}^{T}\*y\vert^{p}+(1/i)^{p/2-1}(1-\vert \tilde{\*u}_{i}^{T}\*y\vert^{2})^{p/2}}$. Note that this function increases with value of $|\tilde{\*u}_{i}^{T}\*y|$, which is maximum when $\*y = \frac{\tilde{\*u}_{i}}{\norm{\tilde{\*u}_{i}}}$,
\begin{equation}
 \tilde{s}_{i} \leq \frac{\norm{\tilde{\*u}_{i}}^{p}}{\norm{\tilde{\*u}_{i}}^{p} + (1/i)^{p/2-1}(1-\norm{\tilde{\*u}_{i}}^{2})^{p/2}} \nonumber
\end{equation}
We know that a function $\frac{a}{a+b} \leq \min\{1,a/b\}$, so we get $\tilde{l}_{i} = \min\{1,i^{p/2-1}\norm{\tilde{\*u}_{i}}^{p}\}$. Note that $\tilde{l}_{i} = i^{p/2-1}\norm{\tilde{\*u}_{i}}^{p}$ when $\norm{\tilde{\*u}_{i}}^{p} < (1/i)^{p/2-1}$ and it implies that $(1-\|\tilde{\*u}_{i}\|^{2})$ close to $1$.
% Now we consider 2 cases,
% \noindent\paragraph{Case 1:} Here we consider for rows with $\norm{\tilde{\*u}_{i}}^{p} < (1/i)^{p/2-1}$. Here each $S_{i} \leq i^{p/2-1}\norm{\tilde{\*u}_{i}}^{p}$. 
% \noindent\paragraph{Case 2:} Here we consider for rows with $\norm{\tilde{\*u}_{i}}^{p} \geq (1/i)^{2/p-1}$. Then each $S_{i} = 1$. 
% 
\end{proof}
Here the scores are similar to leverage scores \cite{woodruff2014sketching} but due to $p$ order and data point coming in online manner the algorithm changes $i^{p/2-1}$ factor more for every row. Although we have bound on the $\sum_{i}^{n} \tilde{l}_{i}$ from lemma \ref{lemma:onlineSummationBound}, but this factor can be very huge as $i$ increases.
\subsubsection{Proof of Lemma \ref{lemma:onlineGuarantee}}
\begin{proof}{\label{proof:onlineGuarantee}}
 For simplicity we prove this lemma at the last timestamp $n$. But it can also be proved for any timestamp $t_{i}$ which is why the \online~can also be used in restricted streaming (online) setting.
 Now for a fixed $\*x \in \~R^{d}$ and its corresponding $\*y$, we define a random variables as follows, i.e. based on the choice of \online.
 \[ w_{i} =
  \begin{cases}
    \frac{1}{p_{i}}(\*u_{i}^{T}\*y)^{p}  & \quad \text{with probability } p_{i}\\
    0 & \quad \text{with probability } (1-p_{i})
  \end{cases}
\]
Where $\*u_{i}^{T}$ is the $i^{th}$ row of $\*U$ for $[\*U,\Sigma,\*V] = \mbox{svd}(\*A)$ and $\*y = \Sigma\*V^{T}\*x$. Here we get $\~E[w_{i}] = (\*u_{i}^{T}\*y)^{p}$. In our online algorithm we have defined $p_{i} = \min\{r\tilde{l}_{i}/\sum_{j=1}^{i}\tilde{l}_{j},1\}$. When $p_{i}$ is not $1$, we have $p_{i}= r\tilde{l}_{i}/\sum_{j=1}^{i}\tilde{l}_{j}\geq \frac{r|\*u_{i}^{T}\*y|^{p}}{\sum_{j=1}^{i}\tilde{l}_{j}\sum_{j=1}^{i}|\*u_{j}^{T}\*y|^{p}}\geq \frac{r|\*u_{i}^{T}\*y|^{p}}{\sum_{j=1}^{n}\tilde{l}_{j}\sum_{j=1}^{n}|\*u_{j}^{T}\*y|^{p}}$. Now to apply Bernstein \ref{thm:bernstein} we bound the term $\vert w_{i} - \~E[w_{i}]\vert \leq b$. Consider the two possible cases,
 
 \textbf{Case 1:} When $w_{i}$ is non zero, then $|w_{i} - \~E[w_{i}]| \leq |w_{i}| \leq \frac{|\*u_{i}^{T}\*y|^{p}}{p_{i}} \leq \frac{|\*u_{i}^{T}\*y|^{p}(\sum_{j=1}^{n} \tilde{l}_{j})\sum_{j=1}^{n} |\*u_{j}^{T}\*y|^{p}}{r|\*u_{i}^{T}\*y|^{p}} = \frac{(\sum_{j=1}^{n} \tilde{l}_{j})\sum_{j=1}^{n} |\*u_{j}^{T}\*y|^{p}}{r}$. Note for $p_{i}=1, \vert w_{i} - \~E[w_{i}]\vert = 0$.
 
 \textbf{Case 2} When $w_{i}$ is $0$ then $p_{i} < 1$. So we have $1 > \frac{r\tilde{l}_{i}}{\sum_{j=1}^{i}\tilde{l}_{j}} \geq \frac{r|\*u_{i}^{T}\*y|^{p}}{(\sum_{j=1}^{n} \tilde{l}_{j})\sum_{j=1}^{n}|\*u_{j}^{T}\*y|^{p}}$. So $\vert w_{i}-\~E[w_{i}]\vert = |\~E[w_{i}|] = |\*u_{i}^{T}\*y|^{p} < \frac{(\sum_{j=1}^{n} \tilde{l}_{j})\sum_{j=1}^{n} |\*u_{j}^{T}\*y|^{p}}{r}$. 
 
 So $b=\frac{(\sum_{j=1}^{n} \tilde{l}_{j})\sum_{j=1}^{n} |\*u_{j}^{T}\*y|^{p}}{r}$. Next we bound the variance of the sum $\sum_{i=1}^{n} \tilde{l}_{i}$. Let $\sigma^{2} = \mbox{var}\big(\sum_{i=1}^{n} w_{i}\big) = \sum_{i=1}^{n} \sigma_{i}^{2}$, where $\sigma_{i}^{2} = \mbox{var}(w_{i})$
% (Online) Further we bound the variance of the sum of random variables till $i$. Let $\mbox{var}_{i} = \mbox{var}\bigg(\sum_{j=1}^{i} w_{j}\bigg)$
 \begin{eqnarray}
  \sigma^{2} = \sum_{i=1}^{n} \sigma_{i}^{2} &=& \sum_{i=1}^{n} \~E[w_{i}^{2}] - (\~E[w_{i}])^{2} \nonumber \\
  &=& \sum_{i=1}^{n}\frac{|\*u_{i}^{T}\*y|^{2p}}{p_{i}} \nonumber \\
  &\leq& \sum_{i=1}^{n}\frac{|\*u_{i}^{T}\*y|^{2p}(\sum_{k=1}^{n} \tilde{l}_{k})\sum_{j=1}^{n} |\*u_{j}^{T}\*y|^{p}}{r|\*u_{i}^{T}\*y|^{p}} \nonumber \\
  &\leq& \frac{(\sum_{k=1}^{n} \tilde{l}_{k})(\sum_{j=1}^{n} |\*u_{j}^{T}\*y|^{p})^{2}}{r} \nonumber
 \end{eqnarray}
%  While first inequality is by definition of variance, the second equation is the expected value. The third inequality is for those $i$'s whose corresponding $p_{i}$'s are strictly less than $1$, as variance for $i$'s with $p_{i}=1$ would be $0$. 
 Note that $\|\*U\*y\|_{p}^{p} = \sum_{j=1}^{n} |\*u_{j}^{T}\*y|^{p}$, now setting $t = \epsilon \sum_{j=1}^{n} |\*u_{j}^{T}\*y|^{p}$, let 
 $$\~P = \mbox{Pr}\bigg(|W - \sum_{j=1}^{n} (\*u_{j}^{T}\*y)^{p}| \geq \epsilon \sum_{j=1}^{n} |\*u_{j}^{T}\*y|^{p}\bigg)$$
 \begin{eqnarray}
  \~P &\leq& \exp\bigg(\frac{\big(\epsilon \sum_{j=1}^{n} |\*u_{j}^{T}\*y|^{p}\big)^{2}}{2\sigma^{2}+bt/3}\bigg) \nonumber \\ 
%   &\leq& \exp\Bigg(\frac{-\epsilon^{2}(\|\*U\*y\|_{p}^{p})^{2}}{2\sum_{j=1}^{n}\tilde{l}_{j}(\|\*U\*y\|_{p}^{p})^{2}/r+ \epsilon\sum_{j=1}^{n}\tilde{l}_{j}(\|\*U\*y\|_{p}^{p})^{2}/3r} \Bigg) \nonumber\\
  &\leq& \exp\Bigg(\frac{-r\epsilon^{2}(\|\*U\*y\|_{p}^{p})^{2}}{(\|\*U\*y\|_{p}^{p})^{2}\sum_{j=1}^{n}\tilde{l}_{j}(2+\epsilon/3)}\Bigg) \nonumber \\
  &=& \exp\Bigg(\frac{-r\epsilon^{2}}{(2+\epsilon/3)\sum_{j=1}^{n}\tilde{l}_{j}}\Bigg) \nonumber
 \end{eqnarray}
 Now to ensure that the above probability at most $\delta$ we need to set $r = \frac{2k\sum_{j=1}^{n}\tilde{l}_{j}} {\epsilon^{2}} \log(\frac 1 \delta)$.
 
 Now to ensure the guarantee for $\ell_{p}$ subspace embedding one can define 
 \[ w_{i} =
  \begin{cases}
    \frac{1}{p_{i}}|\*u_{i}^{T}\*y|^{p}  & \quad \text{with probability } p_{i}\\
    0 & \quad \text{with probability } (1-p_{i})
  \end{cases}
 \]
and follow the above proof. By setting the $r = \frac{2k\sum_{j=1}^{n}\tilde{l}_{j}} {\epsilon^{2}} \log(\frac 1 \delta)$ one can get
$$\~P = \mbox{Pr}\bigg(|W - \|\*A\*x\|_{p}^{p}| \geq \epsilon \|\*A\*x\|_{p}^{p}\bigg) \leq \delta$$
One may follow the above proof to claim the final guarantee in equation \ref{eq:lp} using the same sampling complexity.
\end{proof}
Now give the detail proof of sum of upper bounds of sensitivity scores.
\subsubsection{Proof of Lemma \ref{lemma:onlineSummationBound}}
\begin{proof}{\label{proof:onlineSummationBound}}
Recall that $\*A_i$ denotes the $i\times d$ matrix of the first $i$ vectors. \online~maintains the covariance matrix $\*M$. At the $(i-1)^{th}$ step we have $\*M = \*A_{i-1}^T\*A_{i-1}$. This is then used to define the score $\tilde{l}_{i}$  for the next step $i$, as $\tilde{l}_i = \min\{i^{p/2-1}\tilde{e}_{i}^{p/2},1\}$, where $\tilde{e}_i = \*a_{i}^T (\*A_{i}^T \*A_{i})^{\dagger} \*a_{i}$ and $\*a_{i}^{T}$ is the $i^{th}$ row. 
The scores $\tilde{e}_{i}$ are also called online leverage scores. We first give a bound on $\sum_{i=1}^{n} \tilde{e}_{i}$. A similar bound is given in the online matrix row sampling by~\cite{cohen2016online}, albeit for a regularized version of the scores $\tilde{e}_i$. 
As the rows are coming, the rank of $\*M$ increases 
from $1$ to at most $d$. We say that the algorithm is
in phase-$k$ if the rank of $\*M$ equals $k$. For each phase $k \in [1, d-1]$, let $i_k$ denote the index
where row $a_{i_k}$ caused a phase-change in $\*M$ i.e. 
rank of $(\*A_{i_k-1}^{T} \*A_{i_k-1})$ is $k-1$, while rank of $(\*A_{i_k}^{T} \*A_{i_k})$ is $k$. 
For each $i_k$, the leverage score $\tilde{e}_{i_k} = 1$, since row $\*A_{i_k}$
does not lie in the space of rows $\mathbf{a_1},\ldots, \mathbf{a_{i_k - 1}}$. There
are at most $d$ such indices $i_k$.

We now bound the $\sum_{i\in [i_k, i_{k+1}-1]} \tilde{e}_i$. Suppose the $\mbox{thin-SVD}(\*A_{i_k}^T \*A_{i_k})=\*V\mathbf{\Sigma_{i_k}} \*V^T$, all entries in $\mathbf{\Sigma_{i_k}}$ being positive. 
Furthermore, for any $i$ in this phase, i.e. for $i\in [i_{k}, i_{k+1}-1]$, $\*V$ forms the basis of the row space of $\*A_{i}$. Define
$\*X_{i} = \*V^T (\*A_{i}^T \*A_{i}) \*V$ and $\*a_{i} = \*V \*b_{i}$. Notice that each $\*X_{i}\in \Re^{k\times k}$, and $\*X_{i_k} = \mathbf{\Sigma_{i_k}}$. Also, $\*X_{i_k}$ is positive definite and hence full rank for each $i\in [i_{k}, i_{k+1}-1]$. We also have $\*X_{i} = \*X_{i-1} + \*b_{i} \*b_{i}^T$.

So we have, $\tilde{e}_{i} = \*a_{i}^T(\*A_{i}^T \*A_{i} )^{\dagger}\*a_{i} = \*b_{i}^T\*V^T(\*V(\mathbf{\Sigma_{i-1}}+\*b_{i} \*b_{i}^T)\*V^T)^{\dagger}\*V \*b_{i}=  \*b_{i}^T(\*X_{i-1}+\*b_{i}\*b_{i}^T)^{\dagger}\*b_{i} = \*b_{i}^T(\*X_{i-1}+\*b_{i}\*b_{i}^T)^{-1}\*b_{i}$
where the last equality uses the invertibility of the matrix. 
%  
% Note that matrix $\mathbf{\Sigma_{i-1}}+\*b_{i}\*b_{i}^T$ is a positive definite and hence a full rank matrix. 
 Now using matrix determinant lemma~\cite{vrabel2016note} on
 $\mbox{det}(\*X_{i-1}+\*b_{i}\*b_{i}^T)$ we get,
 \begin{eqnarray*}
  &=& \mbox{det}(\*X_{i-1})(1+\*b_{i}^T(\*X_{i-1})^{-1}\*b_{i}) \nonumber \\
  &\stackrel{(i)}{\geq}& \mbox{det}(\*X_{i-1})(1+\*b_{i}^T(\*X_{i-1}+\*b_{i} \*b_{i}^T)^{-1}\*b_{i}) \nonumber \\
  &=& \mbox{det}(\*X_{i-1})(1+\tilde{e}_{i}) \nonumber \\
  &\stackrel{(ii)}{\geq}& \mbox{det}(\*X_{i-1})\exp(\tilde{e}_{i}/2) \nonumber \\
  \exp(\tilde{e}_{i}/2) &\leq& \frac{\mbox{det}(\*X_{i-1}+\*b_{i}\*b_{i}^T)}{\mbox{det}(\*X_{i-1})} \nonumber
 \end{eqnarray*}
 Inequality $(i)$ follows as $\*X_{i-1}^{-1} - (\*X_{i-1} + \*b\*b^T)^{-1}\succeq 0$ (i.e. p.s.d.). Inequality $(ii)$ follows from
 the fact that $1+x \ge \exp(x/2)$ for $x \leq 1$ and by definition $\tilde{e}_{i} \leq 1$. Now since $\tilde{e}_{i_k} =1$, we analyze
%  \begin{align*}
%      \prod_{i\in[i_k+1, i_{k+1}-1]} \exp(\tilde{e}_{i}/2)  &\le  \prod_{i\in[i_k+1, i_{k+1}-1]}  \frac{\mbox{det}(X_{i})}{\mbox{det}(\*X_{i-1})} \le \frac{\mbox{det}(\mathbf{X_{i_{k+1}-1}})}{\mbox{det}(\*X_{i_k})}.
%  \end{align*}
 \begin{align*}
     \prod_{i\in[i_k+1, i_{k+1}-1]} \exp(\tilde{e}_{i}/2)  &\le  \prod_{i\in[i_k+1, i_{k+1}-1]}  \frac{\mbox{det}(\*X_{i})}{\mbox{det}(\*X_{i-1})}\\ &\le \frac{\mbox{det}(\mathbf{X_{i_{k+1}-1}})}{\mbox{det}(\mathbf{X_{i_k+1}})}.
 \end{align*}
 Taking the product over all the phases $\exp\bigg(\sum_{i\in [1, i_{d}-1]} \tilde{e}_{i}/2\bigg)$ gets,
%  \begin{align*}
%  \exp\bigg(\sum_{i\in [1, i_{d}-1]} \tilde{e}_{i}/2\bigg) & = \prod_{k\in [1,d-1]} \prod_{i\in[i_k+1, i_{k+1}-1]} \exp(\tilde{e}_{i}/2) \\
%  & =  \prod_{k\in [1,d-1]}\frac{\mbox{det}(\mathbf{X_{i_{k+1}-1}})}{\mbox{det}(\*X_{i_k})} =  \frac{\mbox{det}(\mathbf{X_{i_{d}-1}})}{\mbox{det}(X_{i_{1}})}\prod_{k\in [2,d-2]} \frac{\mbox{det}(\mathbf{X_{i_{k+1}-1}})}{\mbox{det}(X_{i_{k+1}})}
%  \end{align*}
\begin{align*}
 & = \exp((d-1)/2)\Big(\prod_{k\in [1,d-1]} \prod_{i\in[i_k+1, i_{k+1}-1]} \exp(\tilde{e}_{i}/2)\Big) \\
 & =  \exp((d-1)/2)\Big(\prod_{k\in [1,d-1]}\frac{\mbox{det}(\mathbf{X_{i_{k+1}-1}})}{\mbox{det}(\mathbf{X_{i_k+1}})}\Big)  \\ &=  \exp((d-1)/2)\Big(\frac{\mbox{det}(X_{i_{2}-1})}{\mbox{det}(X_{i_{1}})}\prod_{k\in [2,d-1]} \frac{\mbox{det}(\mathbf{X_{i_{k+1}-1}})}{\mbox{det}(\mathbf{X_{i_k+1}})}\Big)
 \end{align*}
 Because we know that $(\mathbf{A_{i_{k+1}-1}}^T \mathbf{A_{i_{k+1}-1}}) \succeq (\mathbf{A_{i_k+1}}^T \mathbf{A_{i_k+1}})$ so we get,
 $\mbox{det}(\mathbf{A_{i_{k+1}-1}}^T \mathbf{A_{i_{k+1}-1}}) \ge \mbox{det}(\mathbf{A_{i_k+1}}^T \mathbf{A_{i_k+1}})$. We get $\exp((d-1)/2)$ as there are $d-1$ many $i$ such that $\tilde{e}_{i} =1$. Hence, 
 \begin{align*}
     \exp\bigg(\sum_{i\in [1, i_{d}-1]} \tilde{e}_{i}/2\bigg) &\le \frac{\exp((d-1)/2)\mbox{det}(\mathbf{X_{i_{d}-1}})}{\mbox{det}(\mathbf{X_{i_1+1}})}\\ 
     &\le \frac{\exp((d-1)/2)\mbox{det}(\mathbf{A_{i_d}}^T \mathbf{A_{i_d}})}{\mbox{det}(\mathbf{X_{i_1+1}})}.
 \end{align*}
 Furthermore, we know $\tilde{e}_{i_d}=1$ so for $i\in [i_d, n]$, the matrix $\*M$ is full rank. We follow the same argument as above, and obtain
 \begin{align*}
 \exp\bigg(\sum_{i\in [i_d, n]} \tilde{e}_{i}/2\bigg) &\le \frac{\exp(1/2)\mbox{det}(\*A^T \*A)}{\mbox{det}(\mathbf{A_{i_d+1}}^T \mathbf{A_{i_d+1}})}\\
 & \le \frac{\exp(1/2)\|\*A\|^d}{\mbox{det}(\mathbf{A_{i_d+1}}^T \mathbf{A_{i_d+1}})} 
 \end{align*}
Let $\mathbf{a_{1}}$ be the first incoming row. Now multiplying the above two expressions and taking logarithm of both sides, and accounting for the indices $i_k$ for $k\in[2,d]$,
\begin{align*}
    \sum_{i\le n} \tilde{e}_i &\le d/2 + 2 d\log\|\*A\| - 2\log \|\*a_{1}\| \\
    &\le d/2 + 2 d\log\|\*A\| - \min_{i}2\log \|\*a_{i}\|. 
\end{align*}
Now, we give a bound on $\sum_{i=1}^{n} \tilde{l}_{i}$ where $\tilde{l}_{i} = \min\{1,i^{p/2-1}\tilde{e}_{i}^{p/2}\} \leq \min\{1,n^{p/2-1}\tilde{e}_{i}^{p/2}\}$. We consider two cases. When $\tilde{e}_i^{p/2} \geq n^{1-p/2}$ then $\tilde{l}_{i} = 1$, this implies that $\tilde{e}_i \geq n^{2/p-1}$. But we know $\sum_{i=1}^{n} \tilde{e}_i 
\le O(d+d\log\|\*A\|-\min_{i}\log \|\*a_{i})\|$ and hence there are at-most $O(n^{1-2/p}(d+d\log\|\*A\|-\min_{i}\log \|\*a_{i}\|))$ indices such $\tilde{l}_{i} = 1$. Now for the case where $\tilde{e}_{i}^{p/2} < n^{1-p/2}$, we get $\tilde{e}_{i}^{p/2-1} \leq (n)^{(1-p/2)(1-2/p)}$. Then $\sum_{i=1}^{n} n^{p/2-1}\tilde{e}_{i}^{p/2} = \sum_{i=1}^{n} n^{p/2-1}\tilde{e}_{i}^{p/2-1} \tilde{e}_{i} \leq \sum_{i=1}^{n}n^{1-2/p}\tilde{e}_{i}$ is $O(n^{1-2/p}(d+d\log\|\*A\|-\min_{i}\log \|\*a_{i}\|))$.
\end{proof}
\subsection{\online+\mrlw}
As we know that any offline algorithm can be converted into a streaming algorithm by using merge and reduce method~\cite{har2004coresets}, so we apply merge and reduce on \cite{cohen2015p}. Now we discuss the guarantee that we get from the streaming version of \cite{cohen2015p}.
\subsubsection{Proof of Lemma \ref{lemma:Stream-MR}}
\begin{proof}\label{proof:Stream-MR}
 Here the data is coming in streaming sense and it is feed to the streaming version of the algorithm in \cite{cohen2015p} for $\ell_{p}$ subspace embedding. We use merge and reduce from \cite{har2004coresets} for streaming data. We call it \mrlw~. From \cite{cohen2015p} We know that for a set $\*P$ of size $n$ takes $O(nd^{p/2})$ time to return a coreset $\*Q$ of size $O(d^{p/2}(\log d)(\log 1/\epsilon)\epsilon^{-5})$. Note that for the \mrlw~in section 7 of \cite{har2004coresets} we set $M=O(d^{p/2}(\log d)(\log 1/\epsilon)\epsilon^{-5})$. The method returns $\*Q_{i}$ as the $(1 + \delta_{i})$ coreset for the partition $\*P_{i}$ where $|\*P_{i}|$ is either $2^{i}M$ or $0$, here $\rho_{j} = \epsilon/(c(j+1)^{2})$ such that $1+\delta_{i} = \prod_{j=0}^{i} (1 + \rho_{j}) \leq 1 + \epsilon/2, \forall j \in \lceil \log n \rceil$. Thus we have $|\*Q_{i}|$ is $O(d^{p/2}(\log d)(\log 1/\epsilon)(i+1)^{10}\epsilon^{-5})$. In \mrlw~the method reduce sees at max $\log n$ many coresets at any point of time. Hence the total working space is $O(d^{p/2}(\log^{11} n)(\log d)(\log 1/\epsilon)\epsilon^{-5})$. Now the amortized time spent per update is,
 \begin{eqnarray*}
  && \sum_{i=1}^{\lceil \log (n/M) \rceil} \frac{1}{2^{i}M}(|\*Q_{i}|d^{p/2}) \\
  &=& \sum_{i=1}^{\lceil \log (n/M) \rceil} \frac{1}{2^{i}M}(M(i+1)^{4}d^{p/2}) \leq d^{p/2}
 \end{eqnarray*}
So the finally the algorithm return $\*Q$ as the final coreset of $O(d^{p/2}(\log^{10} n)(\log d)(\log 1/\epsilon)\epsilon^{-5})$ rows and uses $O(d^{p/2})$ ammortized update time.
\end{proof}
Next we discuss the guarantee that we get by feeding the output of \online~to \mrlw~of \cite{cohen2015p}
\subsubsection{Proof of Theorem \ref{thm:improvedStream-MR}}
\begin{proof}\label{proof:improvedStream-MR}
 Here the data is coming in streaming sense. Now \online~filters out the rows with small sensitivity scores and only the sampled rows (high sensitivity score) are feed to \mrlw. We know that for a set $\*P$ of size $n$ takes $O(nd^{p/2})$ time to return a coreset $\*Q$ of size $O(d^{p/2}(\log d)(\log 1/\epsilon)\epsilon^{-5})$ by \cite{cohen2015p}. But here the \online~ensures that \mrlw~only gets $\tilde{O}(n^{1-2/p}d)$, hence the amortized update time is same as that of \online, i.e. $O(d^{2})$. Now similar to the above proof \ref{proof:improvedStream-MR}, by the \mrlw~from section 7 of \cite{har2004coresets} we set $M=O(d^{p/2}(\log d)(\log 1/\epsilon)\epsilon^{-5})$. The method returns $\*Q_{i}$ as the $(1 + \delta_{i})$ coreset for the partition $\*P_{i}$ where $|\*P_{i}|$ is either $2^{i}M$ or $0$, here $\rho_{j} = \epsilon/(c(j+1)^{2})$ such that $1+\delta_{i} = \prod_{j=0}^{i} (1 + \rho_{j}) \leq 1 + \epsilon/2, \forall j \in \lceil \log n \rceil$. Thus we have $|\*Q_{i}|$ is $O(d^{p/2}(\log d)(\log 1/\epsilon)(i+1)^{10}\epsilon^{-5})$. Hence the total working space is $O((1-2/p)^{11}d^{p/2}(\log^{11} n)(\log d)(\log 1/\epsilon)\epsilon^{-5})$. So finally \online+\mrlw~returns a coreset $\*Q$ of $O((1-2/p)^{10}d^{p/2}(\log^{10} n)(\log d)(\log 1/\epsilon)\epsilon^{-5})$ rows.
\end{proof}
\subsection{\kernelfilter}
In this section we discuss the supporting lemma for proving the theorem~\ref{thm:slowOnline}. 
\subsection{Proof of Lemma~\ref{lemma:kernel}}
\begin{proof}{\label{proof:kernel}}
The term $|\*x^{T}\*y|^{p}=|\*x^{T}\*y|^{\lfloor p/2 \rfloor}|\*x^{T}\*y|^{\lceil p/2 \rceil}$. We define $|\*x^{T}\*y|^{\lfloor p/2 \rfloor} = |\grave{\*a}_{i}^{T}\grave{\*x}|$ and $|\*x^{T}\*y|^{\lceil p/2 \rceil} = |\acute{\*a}_{i}^{T}\acute{\*x}|$. For even valued $p$ we know $\lfloor p/2 \rfloor=\lceil p/2 \rceil$, so for simplicity we write as $|\*x^{T}\*y|^{p/2} = |\hat{\*a}_{i}^{T}\hat{\*x}|$. So we get $|\*x^{T}\*y|^{p} = |\langle \*x \otimes^{p/2}, \*y \otimes^{p/2} \rangle|^{2} = |\hat{\*x}^{T}\hat{\*y}|^{2}$. Here the vector $\hat{\*x} = \mbox{vec}(\*x \otimes^{p/2}) \in \~R^{p/2}$ and similarly $\hat{\*y}$ is also defined. Now for odd value of $p$ we have $\grave{\*x} = \mbox{vec}(\*x \otimes^{(p-1)/2}) \in \~R^{(p-1)/2}$ and $\acute{\*x} = \mbox{vec}(\*x \otimes^{(p+1)/2}) \in \~R^{(p+1)/2}$. Similarly $\grave{\*y}$ and $\acute{\*y}$ are defined for odd value of $p$. So we get $|\*x^{T}\*y|^{p} = |\langle \*x \otimes^{(p-1)/2}, \*y \otimes^{(p-1)/2} \rangle|\cdot|\langle \*x \otimes^{(p+1)/2}, \*y \otimes^{(p+1)/2} \rangle| = |\grave{\*x}^{T}\grave{\*y}|\cdot|\acute{\*x}^{T}\acute{\*y}|$.
\[|\*x^{T}\*y|^{p} =
  \begin{cases}
  |\hat{\*x}^{T}\hat{\*y}|^{2}  & \quad \text{if } p \mbox{ even}\\
  |\grave{\*x}^{T}\grave{\*y}|\cdot|\acute{\*x}^{T}\acute{\*y}|^{2p/(p+1)}  & \quad \text{if } p\ \mbox{odd}\\
  \end{cases}
\]
\end{proof}
\subsubsection{Proof of Lemma~\ref{lemma:slowOnlineSensitivityBound}}
\begin{proof}{\label{proof:slowOnlineSensitivityBound}}
 We define the online sensitivity scores $\tilde{s}_{i}$ for each point $i$ as follows,
  \allowdisplaybreaks
  \begin{eqnarray*}
  s_{i} &=& \sup_{\{\*x\mid\|\*x\|=1\}}\frac{|\*a_{i}^{T}\*x|^{p}}{\|\*A_{i}\*x\|_{p}^{p}}\\
  &=&\sup_{\{\*x\mid\|\*x\|=1\}}\frac{|\*a_{i}^{T}\*x|^{\lfloor p/2 \rfloor}|\*a_{i}^{T}\*x|^{\lceil p/2 \rceil}}{\|\*A_{i}\*x\|_{p}^{p}} \\
  &=& \sup_{\{\*x,\grave{\*x},\acute{\*x}\mid\|\*x\|=1\}}\frac{|\grave{\*x}^{T}\grave{\*a}_{i}\acute{\*a}_{i}^{T}\acute{\*x}|}{\|\*A_{i}\*x\|_{p}^{p}} \\
  &\stackrel{(i)}=& \sup_{\{\*x,\grave{\*z},\acute{\*z}\mid\|\*x\|=1\}}\frac{|\grave{\*z}^{T}\grave{\*u}_{i}\acute{\*u}_{i}^{T}\acute{\*z}|\cdot(\|\grave{\*z}\|\|\acute{\*z}\|)}{\|\*A_{i}\*x\|_{p}^{p}\cdot(\|\grave{\*z}\|\|\acute{\*z}\|)} \\
  &\stackrel{(ii)}\leq& \sup_{\{\*x,\grave{\*y},\acute{\*y},\grave{\*z},\acute{\*z}\mid\|\*x\|=1\}}\frac{|\grave{\*y}^{T}\grave{\*u}_{i}\acute{\*u}_{i}^{T}\acute{\*y}|\cdot(\|\grave{\*z}\|\|\acute{\*z}\|)}{\|\*A_{i}\*x\|_{p}^{p}} \\
  &\stackrel{(iii)}=& \sup_{\{\*x,\grave{\*y},\acute{\*y},\grave{\*z},\acute{\*z}\mid\|\*x\|=1\}}\frac{|\grave{\*y}^{T}\grave{\*u}_{i}\acute{\*u}_{i}^{T}\acute{\*y}|\cdot\|\grave{\*z}\acute{\*z}^{T}\|}{\|\*A_{i}\*x\|_{p}^{p}} \\
  &\stackrel{(iv)}=& \sup_{\{\*x,\grave{\*y},\acute{\*y}\mid\|\*x\|=1\}}\frac{|\grave{\*y}^{T}\grave{\*u}_{i}\acute{\*u}_{i}^{T}\acute{\*y}|\cdot\|\grave{\Sigma}_{i}\grave{\*V}_{i}^{T}\grave{\*x}\acute{\*x}^{T}\acute{\*V}_{i}\acute{\Sigma}_{i}\|}{\|\*A_{i}\*x\|_{p}^{p}} \\
  &\stackrel{(v)}=& \sup_{\{\*x,\grave{\*y},\acute{\*y}\mid\|\*x\|=1\}}\frac{|\grave{\*y}^{T}\grave{\*u}_{i}\acute{\*u}_{i}^{T}\acute{\*y}| \cdot\|\grave{\*U}_{i}\grave{\Sigma}_{i}\grave{\*V}_{i}^{T}\grave{\*x}\acute{\*x}^{T}\acute{\*V}_{i}\acute{\Sigma}_{i}\acute{\*U}_{i}^{T}\|}{\|\*A_{i}\*x\|_{p}^{p}} \\
  &=& \sup_{\{\*x,\grave{\*y},\acute{\*y}\mid\|\*x\|=1\}}\frac{|\grave{\*y}^{T}\grave{\*u}_{i}\acute{\*u}_{i}^{T}\acute{\*y}|\cdot\|\grave{\*A}_{i}\grave{\*x}\acute{\*x}^{T}\acute{\*A}_{i}^{T}\|}{\|\*A_{i}\*x\|_{p}^{p}} \\
  &\stackrel{(vi)}=& \sup_{\{\*x,\grave{\*y},\acute{\*y}\mid\|\*x\|=1\}}\frac{|\grave{\*y}^{T}\grave{\*u}_{i}\acute{\*u}_{i}^{T}\acute{\*y}|\cdot\mbox{Trace}(\grave{\*A}_{i}\grave{\*x}\acute{\*x}^{T}\acute{\*A}_{i}^{T})}{\|\*A_{i}\*x\|_{p}^{p}} \\
  &\leq& \sup_{\{\*x,\grave{\*y},\acute{\*y}\mid\|\*x\|=1\}}\frac{|\grave{\*y}^{T}\grave{\*u}_{i}\acute{\*u}_{i}^{T}\acute{\*y}|\cdot\big(\sum_{j=1}^{i}|\grave{\*x}^{T}\grave{\*a}_{j}\acute{\*a}_{j}^{T}\acute{\*x}|\big)}{\|\*A_{i}\*x\|_{p}^{p}} \\
  &=& \sup_{\{\*x,\grave{\*y},\acute{\*y}\mid\|\*x\|=1\}}\frac{|\grave{\*y}^{T}\grave{\*u}_{i}\acute{\*u}_{i}^{T}\acute{\*y}|\cdot\|\*A_{i}\*x\|_{p}^{p}}{\|\*A_{i}\*x\|_{p}^{p}} \\
  &=& \sup_{\{\grave{\*y},\acute{\*y}\mid\|\*x\|=1\}}|\grave{\*y}^{T}\grave{\*u}_{i}\acute{\*u}_{i}^{T}\acute{\*y}| \\
  &=& \|\grave{\*u}_{i}\|\cdot\|\acute{\*u}_{i}\|
 \end{eqnarray*}
 Let $\grave{\*A}$ be the matrix where its $j^{th}$ row $\grave{\*a}_{j} = \*a \otimes^{d^{\lfloor p/2 \rfloor}} \in \~R^{d^{\lfloor p/2 \rfloor}}$ and $\acute{\*A}$ be the matrix where its $j^{th}$ row $\acute{\*a}_{j} = \*a \otimes^{d^{\lceil p/2 \rceil}} \in \~R^{d^{\lceil p/2 \rceil}}$. Further let $\grave{\*A}_{i}$ and $\acute{\*A}_{i}$ are the corresponding matrices $\*A_{i} \in \~R^{i \times d}$ which represents first $i$ streaming rows. We define $[\grave{\*U}_{i},\grave{\Sigma}_{i},\grave{\*V}_{i}] = \mbox{svd}(\grave{\*A}_{i})$ such that $\grave{\*a}_{i}^{T} = \grave{\*u}_{i}^{T}\grave{\Sigma}_{i}\grave{\*V}_{i}^{T}$ and $[\acute{\*U}_{i},\acute{\Sigma}_{i},\acute{\*V}_{i}] = \mbox{svd}(\acute{\*A}_{i})$ such that $\acute{\*a}_{i}^{T} = \acute{\*u}_{i}^{T}\acute{\Sigma}_{i}\acute{\*V}_{i}^{T}$. Now for a fixed $\*x \in \~R^{d}$ its corresponding $\grave{\*x}$ and $\acute{\*x}$ are also fixed in their corresponding higher dimensions. Here $\grave{\Sigma}_{i}\grave{\*V}_{i}^{T}\grave{\*x}=\grave{\*z}$ and $\acute{\Sigma}_{i}\acute{\*V}_{i}^{T}\acute{\*x}=\acute{\*z}$ from which we define unit vectors $\grave{\*y} = \grave{\*z}/\|\grave{\*y}\|$ and $\acute{\*y} = \acute{\*z}/\|\acute{\*z}\|$.

 Now The equality (i) is by change of variable where $\grave{\*z}$ and $\acute{\*z}$ are still function of $\*x$ so $\sup$ is still over $\*x$. The (ii) inequality is due to the $\sup$ is over $\grave{\*y}$ and $\acute{\*y}$. Note that $\forall \*x, \exists \grave{\*y}$ and $\exists \acute{\*y}$. The (iii) equality follows by the fact that for any two vector $\*a$ and $\*b$ we know that $\|\*a\|\|\*b\| = \|\*a\*b^{T}\|_{F} = \|\*a\*b^{T}\|$. The (iv) equality is directly by substituting $\grave{\*z}$ and $\acute{\*z}$. The (v) equality follows by adding scale invariant orthonormal column basis $\grave{\*U}$ and $\acute{\*U}$. The (vi) is equality is by the fact that the matrix $\grave{\*A}\grave{\*x}\acute{\*x}^{T}\acute{\*A}^{T}$ is a rank-1 matrix, so we know that the spectral norm is equal to the Frobenius norm of the matrix which is further equal to the trace of the matrix. 

 Note that for even value $p$ we get $\tilde{s}_{i} \leq \|\hat{\*u}_{i}\|^{2}$ as by lemma \ref{lemma:kernel} we get $\grave{\*u}_{i} = \acute{\*u}_{i} = \hat{\*u}_{i}$. In fact this is true because for even $p$ we have $\lfloor p/2 \rfloor = \lceil p/2 \rceil$.
\end{proof}
\subsubsection{Proof of Lemma \ref{lemma:slowOnlineGuarantee}}
\begin{proof}{\label{proof:slowOnlineGuarantee}}
 For simplicity we prove this lemma at the last timestamp $n$. But it can also be proved for any timestamp $t_{i}$ which is why the \kernelfilter~can also be used in restricted streaming (online) setting. Also for a change we show this for $\ell_{p}$ subspace embedding. Now for some fixed $\*x \in \~R^{d}$ we get $\grave{\*x}$ and $\acute{\*x}$. Our algorithm takes the following random variable for every row $i$.
\[ w_{i} =
  \begin{cases}
    (1/p_{i}-1)|\grave{\*x}^{T}\grave{\*a}_{i}\acute{\*a}_{i}^{T}\acute{\*x}|  & \quad \text{w.p. } p_{i}\\
    -|\grave{\*x}^{T}\grave{\*a}_{i}\acute{\*a}_{i}^{T}\acute{\*x}| & \quad \text{w.p. } (1-p_{i})
  \end{cases}
\]
 Now to show the concentration of the expected term we will apply Bernstein's inequality on $W = \sum_{i=1}^{n} w_{i}$. For this first we bound $|w_{i} - \~E[w_{i}]| = |w_{i}|$ as $\~E[w_{i}] = 0$ and then we give a bound on $\mbox{var}(W)$. 

 Now for the $i^{th}$ timestamp if $p_{i}=1$ then $|w_{i}| = 0$, else if $p_{i} <1$ and \kernelfilter~samples the row then $|w_{i}| \leq |\grave{\*x}^{T}\grave{\*a}_{i}\acute{\*a}_{i}^{T}\acute{\*x}|/p_{i} = \|\grave{\*z}\|\|\acute{\*z}\||\grave{\*y}^{T}\grave{\*u}_{i}\acute{\*u}_{i}^{T}\acute{\*y}|/p_{i} \leq \|\grave{\*z}\|\|\acute{\*z}\|\|\grave{\*u}_{i}\|\|\acute{\*u}_{i}\|/(r \|\grave{\*u}_{i}\|\|\acute{\*u}_{i}\|) = \|\grave{\*z}\|\|\acute{\*z}\|/r$. Next when \kernelfilter~does not sample means that $p_{i} < 1$, then $1 > r\|\grave{\*u}_{i}\|\|\acute{\*u}_{i}\| \geq r|\grave{\*y}^{T}\grave{\*u}_{i}\acute{\*u}_{i}^{T}\acute{\*y}|=r|\grave{\*x}^{T}\grave{\*a}_{i}\acute{\*a}_{i}^{T}\acute{\*x}|/ (\|\grave{\*z}\|\|\acute{\*z}\|)$. Finally we get $|\grave{\*x}^{T}\grave{\*a}_{i}\acute{\*a}_{i}^{T}\acute{\*x}| \leq \|\grave{\*z}\|\|\acute{\*z}\|/r$. So for each $i$ we get $|w_{i}| \leq \|\grave{\*z}\|\|\acute{\*z}\|/r \leq \|\*A\*x\|_{p}^{p}$. It is true from the argument analysis \ref{proof:slowOnlineSensitivityBound}.

Next we bound $\sigma^{2} = \mbox{var}(W) = \sum_{i=1}^{n} \mbox{var}(w_{i}) = \sum_{i=1}^{n}\~E[w_{i}^{2}]$ as follows,

\begin{eqnarray*}
 \sigma^{2} &=& \mbox{var}(W) = \sum_{i=1}^{n} \~E[r_{i}^{2}] \\
 &=& \sum_{i=1}^{n} |\grave{\*x}^{T}\grave{\*a}_{i}\acute{\*a}_{i}^{T}\acute{\*x}|^{2}/p_{i} \\
 &=& \sum_{i=1}^{n} \|\grave{\*z}\|\|\acute{\*z}\||\grave{\*y}^{T}\grave{\*u}_{i}\acute{\*u}_{i}^{T}\acute{\*y}||\grave{\*x}^{T}\grave{\*a}_{i}\acute{\*a}_{i}^{T}\acute{\*x}|/p_{i} \\
 &\leq& \|\grave{\*z}\|\|\acute{\*z}\| \|\*A\*x\|_{p}^{p}/r \\
 &\leq& \|\*A\*x\|_{p}^{2p}/r 
%  &\leq& ((\sigma^{\max}_{(p-1)})^{(p-1)}(\sigma^{\max}_{(p+1)})^{(p+1)})^{1/2}\|\*A\*x\|_{p}^{p}/c
\end{eqnarray*}
We obtain the last inequality by similar analysis in \ref{proof:slowOnlineSensitivityBound}. Now we can apply Bernstein \ref{thm:bernstein} on the sum of random variables to bound the event $\~P: \mbox{Pr}(|W| \geq \epsilon\|\*A\*x\|_{p}^{p})$, Here we have $b = \|\*A\*x\|_{p}^{p}/r, \sigma^{2} = \|\*A\*x\|_{p}^{2p}/r$ and we set $t = \epsilon\|\*A\*x\|_{p}^{p}$, then we get
\begin{eqnarray*}
 \~P &\leq& \exp\bigg(\frac{-(\epsilon\|\*A\*x\|_{p}^{p})^{2}}{2\|\*A\*x\|_{p}^{2p}/r+\epsilon\|\*A\*x\|_{p}^{2p}/3r}\bigg) \\
 &=& \exp\bigg(\frac{-r\epsilon^{2}\|\*A\*x\|_{p}^{2p}}{(2+\epsilon/3)\|\*A\*x\|_{p}^{2p}}\bigg) \\
 &=& \exp\bigg(\frac{-r\epsilon^{2}}{(2+\epsilon/3)}\bigg)
\end{eqnarray*}
To ensure the above event with probability at least $1-\delta$ we need to set $r \geq \log(1/\delta)/\epsilon^{-2}$. 

 Now to ensure the guarantee for tensor contraction as equation \eqref{eq:contract} one can define 
 \[ w_{i} =
  \begin{cases}
   (1/p_{i}-1)(\grave{\*x}^{T}\grave{\*a}_{i}\acute{\*a}_{i}^{T}\acute{\*x})  & \quad \text{w.p. } p_{i}\\
   -(\grave{\*x}^{T}\grave{\*a}_{i}\acute{\*a}_{i}^{T}\acute{\*x}) & \quad \text{w.p. } (1-p_{i})
  \end{cases}
 \]
and follow the above proof. By setting the $r = \frac{2k\sum_{j=1}^{n}\tilde{l}_{j}} {\epsilon^{2}} \log(\frac 1 \delta)$ one can get
$$\~P = \mbox{Pr}\bigg(|W - \sum_{j=1}^{n} (\*u_{j}^{T}\*y)^{p}| \geq \epsilon \sum_{j=1}^{n} |\*u_{j}^{T}\*y|^{p}\bigg) \leq \delta$$
One may follow the above proof to claim the final guarantee in equation \ref{eq:contract} using the same sampling complexity.
\end{proof}
\subsubsection{Proof of Lemma \ref{lemma:slowOnlineSummationBound}}
\begin{proof}{\label{proof:slowOnlineSummationBound}}
 Using proof of lemma \ref{lemma:onlineSummationBound}, let $\grave{c}_{i} = \|\grave{\*u}_{i}\|^{2}$ and $\acute{c}_{i} = \|\acute{\*u}_{i}\|^{2}$. Now $\sum_{i=1}^{n} \tilde{l}_{i}\leq\sum_{i=1}^{n}\grave{c}_{i} + \acute{c}_{i}$. From lemma \ref{lemma:onlineSummationBound} we get $\sum_{i=1}^{n} \grave{c}_{i}$ is $O(d^{\lfloor p/2 \rfloor}(1+\log \|\grave{\*A}\|)-\min_{i}\log \|\grave{\*a}_{i}\|)$. Now with $[\*u,\Sigma,\*V] = \mbox{svd}(\*A)$ we have $\grave{\*a}^{T} = \mbox{vec}(\*a_{i}^{T} \otimes^{\lfloor p/2 \rfloor}) = \mbox{vec}((\*u_{i}^{T}\Sigma\*V^{T})^{\lfloor p/2 \rfloor})$. So we get $\|\grave{\*A}\| \leq \sigma_{1}^{\lfloor p/2 \rfloor}$. Hence $\sum_{i=1}^{n}$ is $O(d^{\lfloor p/2 \rfloor}(1+\lfloor p/2 \rfloor\log \|\*A\|)-\lfloor p/2 \rfloor\min_{i}\log \|\*a_{i}\|)$. Similarly we get $\sum_{i=1}^{n} \acute{c}_{i}$ is $O(d^{\lceil p/2 \rceil}(1+\lceil p/2 \rceil\log \|\*A\|)-\lceil p/2 \rceil\min_{i}\log \|\*a_{i}\|)$. So finally $\sum_{i=1}^{n} \tilde{l}_{i}$ is $O(d^{\lceil p/2 \rceil}(1+\lceil p/2 \rceil\log \|\*A\|)-\lfloor p/2 \rfloor\min_{i}\log \|\*a_{i}\|)$.
\end{proof}
\subsection{$p=2$ case}{\label{app:matrix}}
In the following theorem we state the guarantees of our algorithm in the matrix case. 
\begin{corollary}
\label{lem:matrixcoreset}
 Given a matrix $\*A \in \~R^{n\times d}$ with rows coming one at a time, for $p=2$ the algorithm \ref{alg:onlineCoreset} takes $O(d^{2})$ update time and samples $O(\frac{d}{\epsilon^{2}}(d+d\log\|\*A\|-\min_{i}\log \|\*a_{i}\|))$ rows and preserves the following with probability at least 0.9, $\forall \*x \in \~R^{d}$
 $(1-\epsilon)\|\*A\*x\|^{2} \leq \|\*C\*x\|^{2} \leq (1+\epsilon)\|\*A\*x\|^{2}$.
\end{corollary}
Just by using Matrix Bernstein inequality~\cite{tropp2011freedman} we can slightly improve the sampling complexity from $O(d^{2})$ to $O(d\log d)$. For simplicity we modify the sampling probability to $p_{i} = \min\{r\tilde{l}_{i},1\}$ and get the following guarantee.
\begin{theorem}{\label{thm:improvedMatrixCoreset}}
 The above modified algorithm samples $O(\frac{\log d}{\epsilon^{2}}(d+d\log\|\*A\|-\min_{i} \log \|\*a_{i}\|))$ rows and preserves the following with probability at least 0.9, $\forall \*x \in \~R^{d}$
 \begin{align*}
  (1-\epsilon)\|\*A\*x\|^{2} \leq \|\*C\*x\|^{2} \leq (1+\epsilon)\|\*A\*x\|^{2}
 \end{align*}
\end{theorem}
\begin{proof}{\label{proof:improvedMatrixCoreset}}
We prove this lemma in 2 parts. First we show that sampling $\*a_{i}$ with probability $p_{i}=\min\{r\tilde{l}_{i},1\}$ where $\tilde{l}_{i} = \min\{(1+\epsilon)\*a_{i}^{T}(\*A_{i}^{T}\*A_{i})^{\dagger}\*a_{i},1\}$ preserves $\|\*C^{T}\*C\| \leq (1\pm \epsilon)\|\*A^{T}\*A\|, \forall \*x \in \~R^{d}$. Next we give the bound on expected sample size.

We define, $u_{i} = (\*A^{T}\*A)^{-1/2}\*a_{i}$ and we define a random matrix $\*X_{i}$ corresponding to each streaming row as, 
\[ \*X_{i} =
  \begin{cases}
    (1/p_{i} - 1)\*u_{i}\*u_{i}^{T}  & \quad \text{if } \*a_{i} \text{ is sampled in } \tilde{A}\\
    -\*u_{i}\*u_{i}^{T} & \quad \text{else}
  \end{cases}
\]
Now we have,
\begin{eqnarray*}
 \tilde{l}_{i} &=& \*a_{i}^{T}(\*A_{i-1}^{T}\*A_{i-1}+\*a_{i}\*a_{i}^{T})^{\dagger}\*a_{i}\\
 &\geq& \*a_{i}^{T}(\*A^{T}\*A)^{\dagger}\*a_{i}\\
 &=& \*u_{i}^{T}\*u_{i}
\end{eqnarray*}
For $p_{i} \geq \min\{r\*u_{i}^{T}\*u_{i},1\}$, if $p_{i} = 1$, then $\|\*X_{i}\| = 0$, else $p_{i} = r\*u_{i}^{T}\*u_{i} < 1$. So we get $\norm{\*X_{i}} \leq 1/r$. 
Next we bound $\~E[\|\*X_{i}\|^{2}]$.
\begin{eqnarray*}
 \~E[\|\*X_{i}\|^{2}] &=& p_{i}(1/p_{i}-1)^{2}\|\*u_{i}\*u_{i}^{T}\|^{2}+(1-p_{i})\|\*u_{i}\*u_{i}^{T}\|^{2} \\
 &\preceq& \|\*u_{i}\*u_{i}^{T}\|^{2}/p_{i} \\
 &\preceq& \|\*u_{i}\*u_{i}^{T}\|/r
\end{eqnarray*}
Let $\*X = \sum_{i=1}^{n} \*X_{i}$, then variance of $\|\*X\|$ 
\begin{align*}
\mbox{var}(\norm{\*X}) &=& \sum_{i=1}^{n}\mbox{var}(\|\*X_{i}\|) \leq \sum_{i=1}^{n} \~E[\|\*X_{i}\|^{2}] \\
&\leq& \bigg\lVert\sum_{j=1}^{n} \*u_{j}\*u_{j}^{T}/r \bigg\rVert \leq 1/r
\end{align*}
Next by applying matrix Bernstein theorem \ref{thm:matrixBernstein} with appropriate $r$ we get,
$$\mbox{Pr}(\norm{\*X}\geq\epsilon) \leq d \exp\bigg(\frac{-\epsilon^{2}/2}{1/r+\epsilon/(3r)}\bigg)\leq 1/d$$
This implies that the modified algorithm preserves spectral approximation with high probability, i.e. $\norm{\*C^{T}\*C} \leq (1 \pm \epsilon)\norm{\*A^{T}\*A}$.

Now once we have the above result using lemma 4 of \cite{cohen2015uniform} we conclude that the expected number of samples are $O(\sum_{i=1}^{n}\tilde{l}_{i}(\log d)/\epsilon^{2})$. Now from lemma \ref{lemma:onlineSummationBound} we know that for $p=2, \sum_{i=1}^{n}\tilde{l}_{i}$ is $O(d(1+2\log \|\*A\|))$. Finally to get $\mbox{Pr}(\norm{\*X}\geq\epsilon) \leq \delta$ the algorithm samples $O(\frac{d\log d}{\epsilon^{2}}(1+2\log\|\*A\|)\log(1/\delta)$ rows.
\end{proof}
\subsection{Latent Variable Modeling}{\label{sec:application}}
Under the assumption that the data is generated by some generative model such as Gaussian Mixture model, Topic model, Hidden Markov model etc, one can represent the data in terms of higher order moments to realize the latent variables~\cite{anandkumar2014tensor}. Next these higher order moments (Tensors) are reduced to smaller dimensional tensors, which are also orthogonally decomposable. This process is called whitening. For example 
Rephrasing the main theorem 5.1~\cite{anandkumar2014tensor} we get that the $\|\mcal M_{3} - \widetilde{\mcal M}_{3}\| \leq \varepsilon\|\*W\|^{-3}$ where $\mcal M_{3}$ is the true tensor and $\widetilde{\mcal M}_{3}$ is the empirical tensor.
Now we state the guarantees that one gets by applying the RTPI on our sampled data.
\begin{corollary}{\label{coro:tensorFactors}}
 For a dataset with rows coming in streaming fashion and the algorithm \online+\kernelfilter~guarantees \eqref{eq:contract} such that for all unit vector $\*x \in \*Q$, it ensures $\epsilon\sum_{i \leq n} |\*a^{T}\*x|^{3} \leq \varepsilon \|\*W\|^{-3}$. Then applying the RTPI on the sampled coreset $\*C$ returns $k$ eigenpairs $\{\lambda_{i},\*v_{i}\}$ of the reduced (orthogonally decomposable) tensor, ensures that $\forall i \in [k]$,
 $$\|\*v_{\pi(i)} - \*v_{i}\| \leq 8\varepsilon/\lambda_{i} \qquad \qquad |\lambda_{\pi(i)}-\lambda_{i}| \leq 5\varepsilon$$
\end{corollary}
